# Supplementary material for: MOPA: Modular Object Navigation with PointGoal Agents
Source: arXiv:2304.03696 source file (2024-01-27)
Supplement: Supplementary file 1 [file tab-sem-map-exp-suppl.tex]

\begin{table}
    \centering
    \resizebox{\linewidth}{!}{
    \begin{tabular}{@{}lcccccccc@{}}
    \toprule
        & \multicolumn{4}{c}{Validation}                       & \multicolumn{4}{c}{Test} \\
        \cmidrule(l{0pt}r{2pt}){2-5} \cmidrule(l{2pt}r{0pt}){6-9}        & Success  & Progress
         & SPL & PPL & Success  & Progress
         & SPL & PPL \\ 
        \midrule
        CYL & 31 & 47 & 17 & 19 & 27 & 45 & 15 & 17 \\
        NAT & 25 & 37 & 14 & 12 & 20 & 30 & 10 & 17  \\
        \bottomrule
    \end{tabular}}
    \caption{\textbf{\predsem performance on CYL-objects vs NAT-objects} 
    The \predsem agent with Nat-objects performs worse than the one with the CYL-objects. This shows that natural objects with varying sizes, shapes and colors are harder to detect than cylinder objects with same sizes and shapes with varying colors.
    The above set of experiments are on 3ON folds using \pointnav as the \navigation and \randthresh as the \exploration module.}
    \label{tab:sem_map_nat_vs_cyl}
\end{table}
