# Supplementary material for: MOPA: Modular Object Navigation with PointGoal Agents
Source: arXiv:2304.03696 source file (2024-01-27)
Supplement: Supplementary file 2 [file tab-suppl-Nons-full.tex]

\begin{table*}
    \centering
    \resizebox{\linewidth}{!}{
    \begin{tabular}{@{}lllllllllrrrrrrrr@{}}
    \toprule
        &\multirow{2}{*}{\thead{Method}} &\multirow{2}{*}{\thead{Dataset}} &\multirow{2}{*}{\thead{Goals\#}} &\multirow{2}{*}{\thead{Max\\ Steps}} & \multirow{2}{*}{\thead{$\mathcal{O}$}} & \multirow{2}{*}{\thead{$\mathcal{M}$}}  & \multirow{2}{*}{\thead{$\mathcal{N}$}} & \multirow{2}{*}{\thead{$\mathcal{E}$}} & \multicolumn{4}{c}{Validation}                       & \multicolumn{4}{c}{Test} \\
        \cmidrule(l{0pt}r{2pt}){10-13} \cmidrule(l{2pt}r{0pt}){14-17}    
        &&& & &&& & & Success  & Progress
         & SPL & PPL & Success  & Progress
         & SPL & PPL \\ 
         \midrule
        
        1&\multirow{7}{*}{\orasem} &\multirow{5}{*}{\ours} & 1ON &2500 & \oracle & \cite{chaplot2020object} &\pointnavshort & \randthreshshortest  & \textbf{96} & \textbf{96} & \textbf{36} & 36 & \textbf{95} & \textbf{95} & 35 & 35  \\
        2&&&3ON &2500 & \oracle & \cite{chaplot2020object} &\pointnavshort & \randthreshshortest  & 80 & 87 & 35 &\textbf{38}  & 81  & 87  & \textbf{37} & \textbf{39} \\
        3&&&5ON &2500 & \oracle & \cite{chaplot2020object} &\pointnavshort & \randthreshshortest  & 68 & 78 & 33 & 36 & 66 & 76 & 32 & 36 \\
        % \predsem & 1ON & & & & & & & & \\
        % & 3ON & 31 & 47 & 17 & 19 & 27 & 45 & 15 & 17 \\
        % & 5ON & & & & & & & & \\

        4&& & 3ON & 1500 & \oracle & \cite{chaplot2020object} &\pointnavshort & \randthreshshortest  &69 &78 &33 &37 &72 &80 &35 &38 \\

        5&& & 1ON & 500 & \oracle & \cite{chaplot2020object} &\pointnavshort & \randthreshshortest & 69 & 69 &34 &34 &68 &68 &34 &34\\
        
        \cmidrule(l{2pt}r{0pt}){3-17}
        % \midrule        
        6&&\multirow{2}{*}{ObjNav~\cite{habitatchallenge2022}} &1ON &500 & \oracle & \cite{chaplot2020object} &\pointnavshort & \randthreshshortest  &64 &- &30 &- &- &- &- &- \\
        7& & &1ON &500 & \oracle & \cite{chaplot2020object} &\pointnavshort & \frontiershort  &60 &- &28 &- &- &- &- &- \\

         \midrule
       8&  \multirow{2}{*}{\predsem}  &\ours &1ON &500 & \oracle & \cite{chaplot2020object} &\pointnavshort & \randthreshshortest &61 &61  &29  &29  &60  &60  &27  &27  \\
       9&  &ObjNav~\cite{habitatchallenge2022} &1ON &500 & \oracle & \cite{chaplot2020object} &\pointnavshort & \randthreshshortest  &30 &- &28 &- &- &- &- &- \\
    \bottomrule
        \end{tabular}}
    \caption{\textbf{\ours vs ObjectNav.}
    (1) Performance deteriorates as we increase target objects, for a fixed step limit (rows 1-3). 
    (2) Our \orasem performs similarly on the Habitat ObjectNav 2022~\cite{habitatchallenge2022} and \ours 1ON val set (rows 5,6) when we set the step limit to 500 steps, following ObjectNav task setting. (3) In ObjectNav, \orasem performs better (rows 6,7) with \randthresh (\randthreshshortest)  than \frontier (\frontiershort). (4) Our \predsem performs better on \ours than on ObjectNav (rows 8,9).
    }
    \label{tab:suppl_momon_N_ons}
\end{table*}
